# Supplementary material for: How Good Are Coding Agents at Automatic Algorithm Design?
Source: arXiv:2611.36339 source file (2026-11-26)
Supplement: Supplementary file 1 [file hidden_appendix_references.tex]

% Labels from the last full build; hidden appendix references are plain text.
% This file is loaded only when appendices are hidden.
\makeatletter
\newcommand{\reporthiddenappendixlabel}[2]{%
  \expandafter\gdef\csname report@hidden@#1\endcsname{#2}}
\reporthiddenappendixlabel{app:results}{A}
\reporthiddenappendixlabel{app:heldout-expanded}{A}
\reporthiddenappendixlabel{app:test-pfsp}{A.1}
\reporthiddenappendixlabel{app:test-tsp}{A.2}
\reporthiddenappendixlabel{app:test-r18}{A.3}
\reporthiddenappendixlabel{app:test-r20}{A.4}
\reporthiddenappendixlabel{app:development}{B}
\reporthiddenappendixlabel{app:all-trajectories}{B.1}
\reporthiddenappendixlabel{app:execution}{B.2}
\reporthiddenappendixlabel{app:setup}{C}
\reporthiddenappendixlabel{app:instances}{C.1}
\reporthiddenappendixlabel{app:task-example}{C.2}
\reporthiddenappendixlabel{app:environment}{C.3}
\reporthiddenappendixlabel{tab:appendix-pfsp}{26}
\reporthiddenappendixlabel{tab:appendix-tsp}{27}
\reporthiddenappendixlabel{tab:appendix-r18}{28}
\reporthiddenappendixlabel{tab:appendix-r20}{29}

\reporthiddenappendixlabel{app:test-r22}{A.5}
\reporthiddenappendixlabel{tab:appendix-r22-improve}{30}
\reporthiddenappendixlabel{tab:appendix-r22-scratch}{31}

\AddToHook{begindocument/end}{%
\NewCommandCopy\report@linkedref\ref
\RenewDocumentCommand{\ref}{s m}{%
  \ifcsname report@hidden@#2\endcsname
    \csname report@hidden@#2\endcsname
  \else
    \IfBooleanTF{#1}{\report@linkedref*{#2}}{\report@linkedref{#2}}%
  \fi}%
}
\makeatother
